# Supplementary material for: PIM-tree: A Skew-resistant Index for Processing-in-Memory
Source: arXiv:2211.10516 source file (2022-11-18)
Supplement: Supplementary file 1 [file appendix.tex]

% \section{Lemma~\ref{lemma:geometric_balanced} proof}

% \newtheorem*{Lgb}{Lemma~\ref{lemma:geometric_balanced}}
% \begin{Lgb}
%     \wbibt
% \end{Lgb}

% \section{\GET Bounds}
